# Supplementary material for: Kuaipedia: a Large-scale Multi-modal Short-video Encyclopedia
Source: arXiv:2211.00732 source file (2023-08-11)
Supplement: Supplementary file 1 [file appendix.tex]

\clearpage
\appendix
\section{Evaluation Instructions}
\subsection{Aspect Evaluation Instructions} \label{asp-eval-inst}
In order for an aspect to be considered \textbf{meaningful} and \textbf{relevant}, it must meet certain criteria. To be considered meaningful, the aspect must fulfill the following three conditions:

\begin{enumerate}
    \item Validity: The aspect must be a valid word or phrase. For example, ``not a'' or ``baby is'' would not be considered valid.
    \item Core Meanings: The aspect must have independent semantic meanings. Phrases such as ``a lot'' or ``various of'' would not be considered meaningful.
    \item Appropriate Specificity: The aspect should not be too specific, such as an exact count, order, or time frame. For example, ``Step 1'' or ``Task 2'' would not be appropriate aspects.
\end{enumerate}
To be considered relevant, an aspect must meet either of the following two conditions:
\begin{enumerate}
    \item Commonsense Relevancy: The aspect must be related to the item in common sense. For example, the aspect ``ear'' would be considered relevant when referring to a ``dog'', but not when referring to a ``bee''.
    \item Popular Relevancy: Although the item and aspect may not be related in common sense, the combination may make sense when searched on the web. For example, ``dog - mental illness'' is relevant because many people search for information on how to alleviate mental illness by petting a dog.

\end{enumerate}

\subsection{Item-aspect Linking Evaluation Instructions} \label{linking-eval-inst}
Here, in order to effectively evaluate the relevance between the item-aspect pair and a short video, we have developed a comprehensive criterion that rates the relevance into four levels (3- Exactly Relevant, 2- Moderately Relevant, 1- Slightly Relevant, 0- Irrelevant). To enhance the accuracy and consistency among human annotators, we have divided the annotation process into two phases. The first phase involves asking annotators to determine the relevance between the video and the item. If the video is found to be discussing the item, we then ask them to determine if the video is discussing a specific aspect of the item. Detailed instructions for these two phases are provided in Table \ref{table:item-relevancy-inst} and Table \ref{table:aspect-relevancy-inst}.

\begin{table*}[!t]
\centering
\begin{tabular}{p{0.2\linewidth} | p{0.75\linewidth}}
\toprule
Score                           & Instructions     \\ 
\midrule
3 - exactly relevant & (1) The video topic aligns with the item topic, either exactly or through the use of synonyms or near-synonyms as long as the meaning is equivalent. The video primarily explains what the item means. For instance, if the item is "astigmatism," the video mainly covers "nearsightedness."; (2)The video topic is somewhat narrower than the item topic, but it covers a significant part or the key aspect of the itme's knowledge. In other words, it satisfies the user's primary information needs. For example, if the item is "early pregnancy," the video focuses on the symptoms of early pregnancy.\\
\midrule
2 - moderately relevant & (1) The theme of the video is more specific than the theme of the item, but the theme of the video is a subcategory of the item. For instance, in the case of "children's songs", the video primarily focuses on the single song "Two Tigers"; (2) Items are generic in nature, and user needs are diverse. Without clear data support, it is challenging to determine the main needs of the user. The video theme can address a specific aspect of the item theme.\\
\midrule
1 - slightly relevant & (1) The video's theme is narrower in scope compared to the theme associated with the item, representing a smaller proportion of the item's intent. To put it differently, it meets the user's secondary intent. For instance, in the case of "children's toys," the video focuses mainly on "Lego."; (2) The theme of the video encompasses a broader range than that of the item, including not only the matching part of the item theme but also the common or natural extensions of the item theme. For example, in the case of "children's clothing," the video provides explanations for children's clothing from ages 0 to 6, but a greater proportion is dedicated to clothing for children over 6. \\
\midrule
0 - irrelevant & (1) When the content of a video is completely inconsistent with the meaning of the item, it is considered to be completely unrelated. For example, if a video discusses "late pregnancy" instead of "early pregnancy" for the item "pregnancy"; (2) If the content of a video only partially satisfies the literal meaning of an item but deviates significantly from the overall meaning of the item and lacks important defining components, it is also considered to be unrelated. For example, if a video only covers "symptoms of childhood diseases" instead of "symptoms of Down syndrome" for the item "symptoms of Down syndrome".\\

\bottomrule
\end{tabular}
\caption{
    The instructions to evaluate the relevancy between the item and the video.
}
\label{table:item-relevancy-inst}
\end{table*}

\begin{table*}[!h]
\centering
\begin{tabular}{p{0.2\linewidth} | p{0.75\linewidth}}
\toprule
Score                           & Instructions     \\ 
\midrule
3 - exactly relevant & (1) The video mainly covers  the aspect, which can be synonyms/near-synonyms as long as the semantics match. For example, if the aspect is ``symptoms of congenital heart disease" and the video mainly discusses ``what are the manifestations" or ``what are the signs" and more than 90\% of the content is about this aspect, it is considered consistent in meaning; (2) The video mainly covers a subset of the aspect. For example, if the aspect is ``prevention and treatment of neonatal jaundice" and the video mainly discusses how to ``prevent" neonatal jaundice, it is considered relevant. \\
\midrule
2 - moderately relevant & (1) The video primarily covers the aspect, with over 60\% of the content dedicated to the specific aspect. For example, the ``how to protect" aspect of the item ``milk teeth," are briefly mentioned in a video, a mention of what to do about tooth decay in the last three seconds of the video would be considered relevant. \\
\midrule
1 - slightly relevant &  The primary objective of the video is to elaborate on the extension of a particular aspect. In this case, the aspect of ``Amniocentesis" and its aspect of ``Inspection". The video focuses on contrasting the differences between non-invasive DNA testing and amniocentesis as means of detecting fetal abnormalities. The content of the video can be considered as partially related to the topic.\\
\midrule
0 - irrelevant & (1) Videos that are completely inconsistent with the aspect are considered completely irrelevant, for example, if the aspect of ``gestational sac" is ``small gestational sac," but the video explains ``large gestational sac."; (2) Videos that only partially meet the literal meaning of the query, but deviate significantly from the overall meaning of the entity term and lose important qualifying components, are also deemed irrelevant. For example, if the entity term is ``Down syndrome," and the aspect is the symptoms, but the video explains the content related to ``Down syndrome screening," it would be considered irrelevant. \\

\bottomrule
\end{tabular}
\caption{
    The instructions to evaluate the relevancy between the aspect and the video.
}
\label{table:aspect-relevancy-inst}
\end{table*}

\begin{figure*}[h]
\centering
\includegraphics[width=1.0\textwidth]{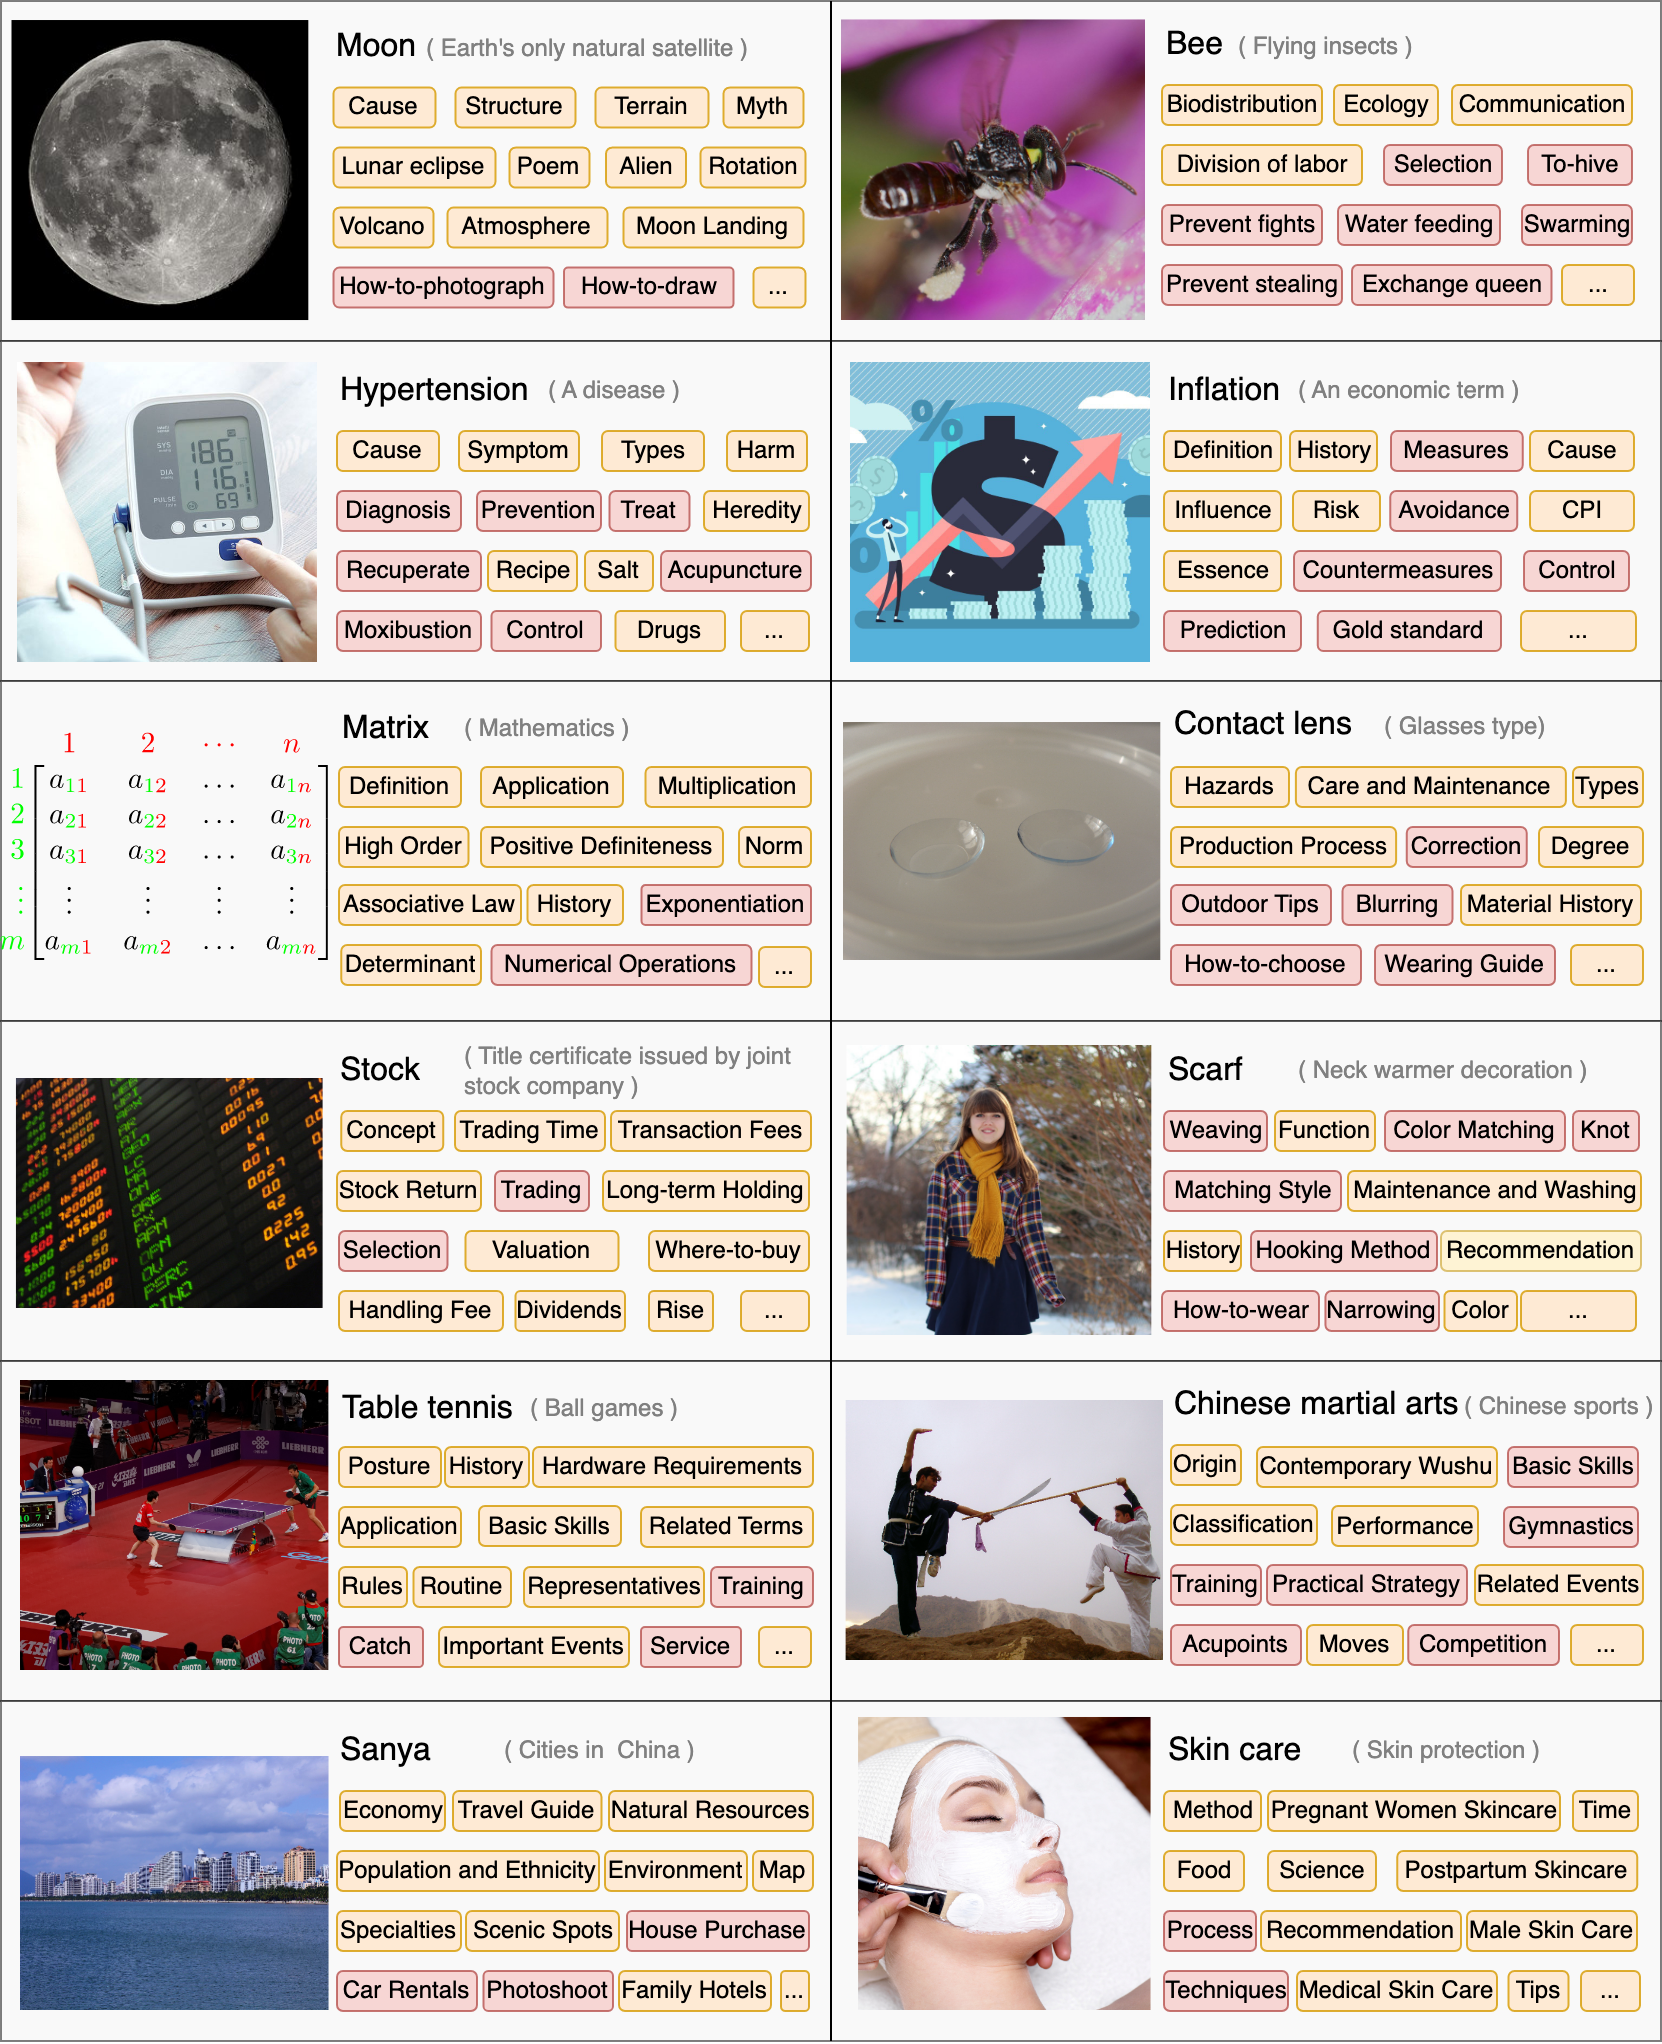}
\caption{More cases of Item-aspect pairs in Kuaipedia.}
\label{fig:aspect-case-appendix}
\end{figure*}

\begin{figure*}[h]
\centering
\includegraphics[height=0.6\textwidth]{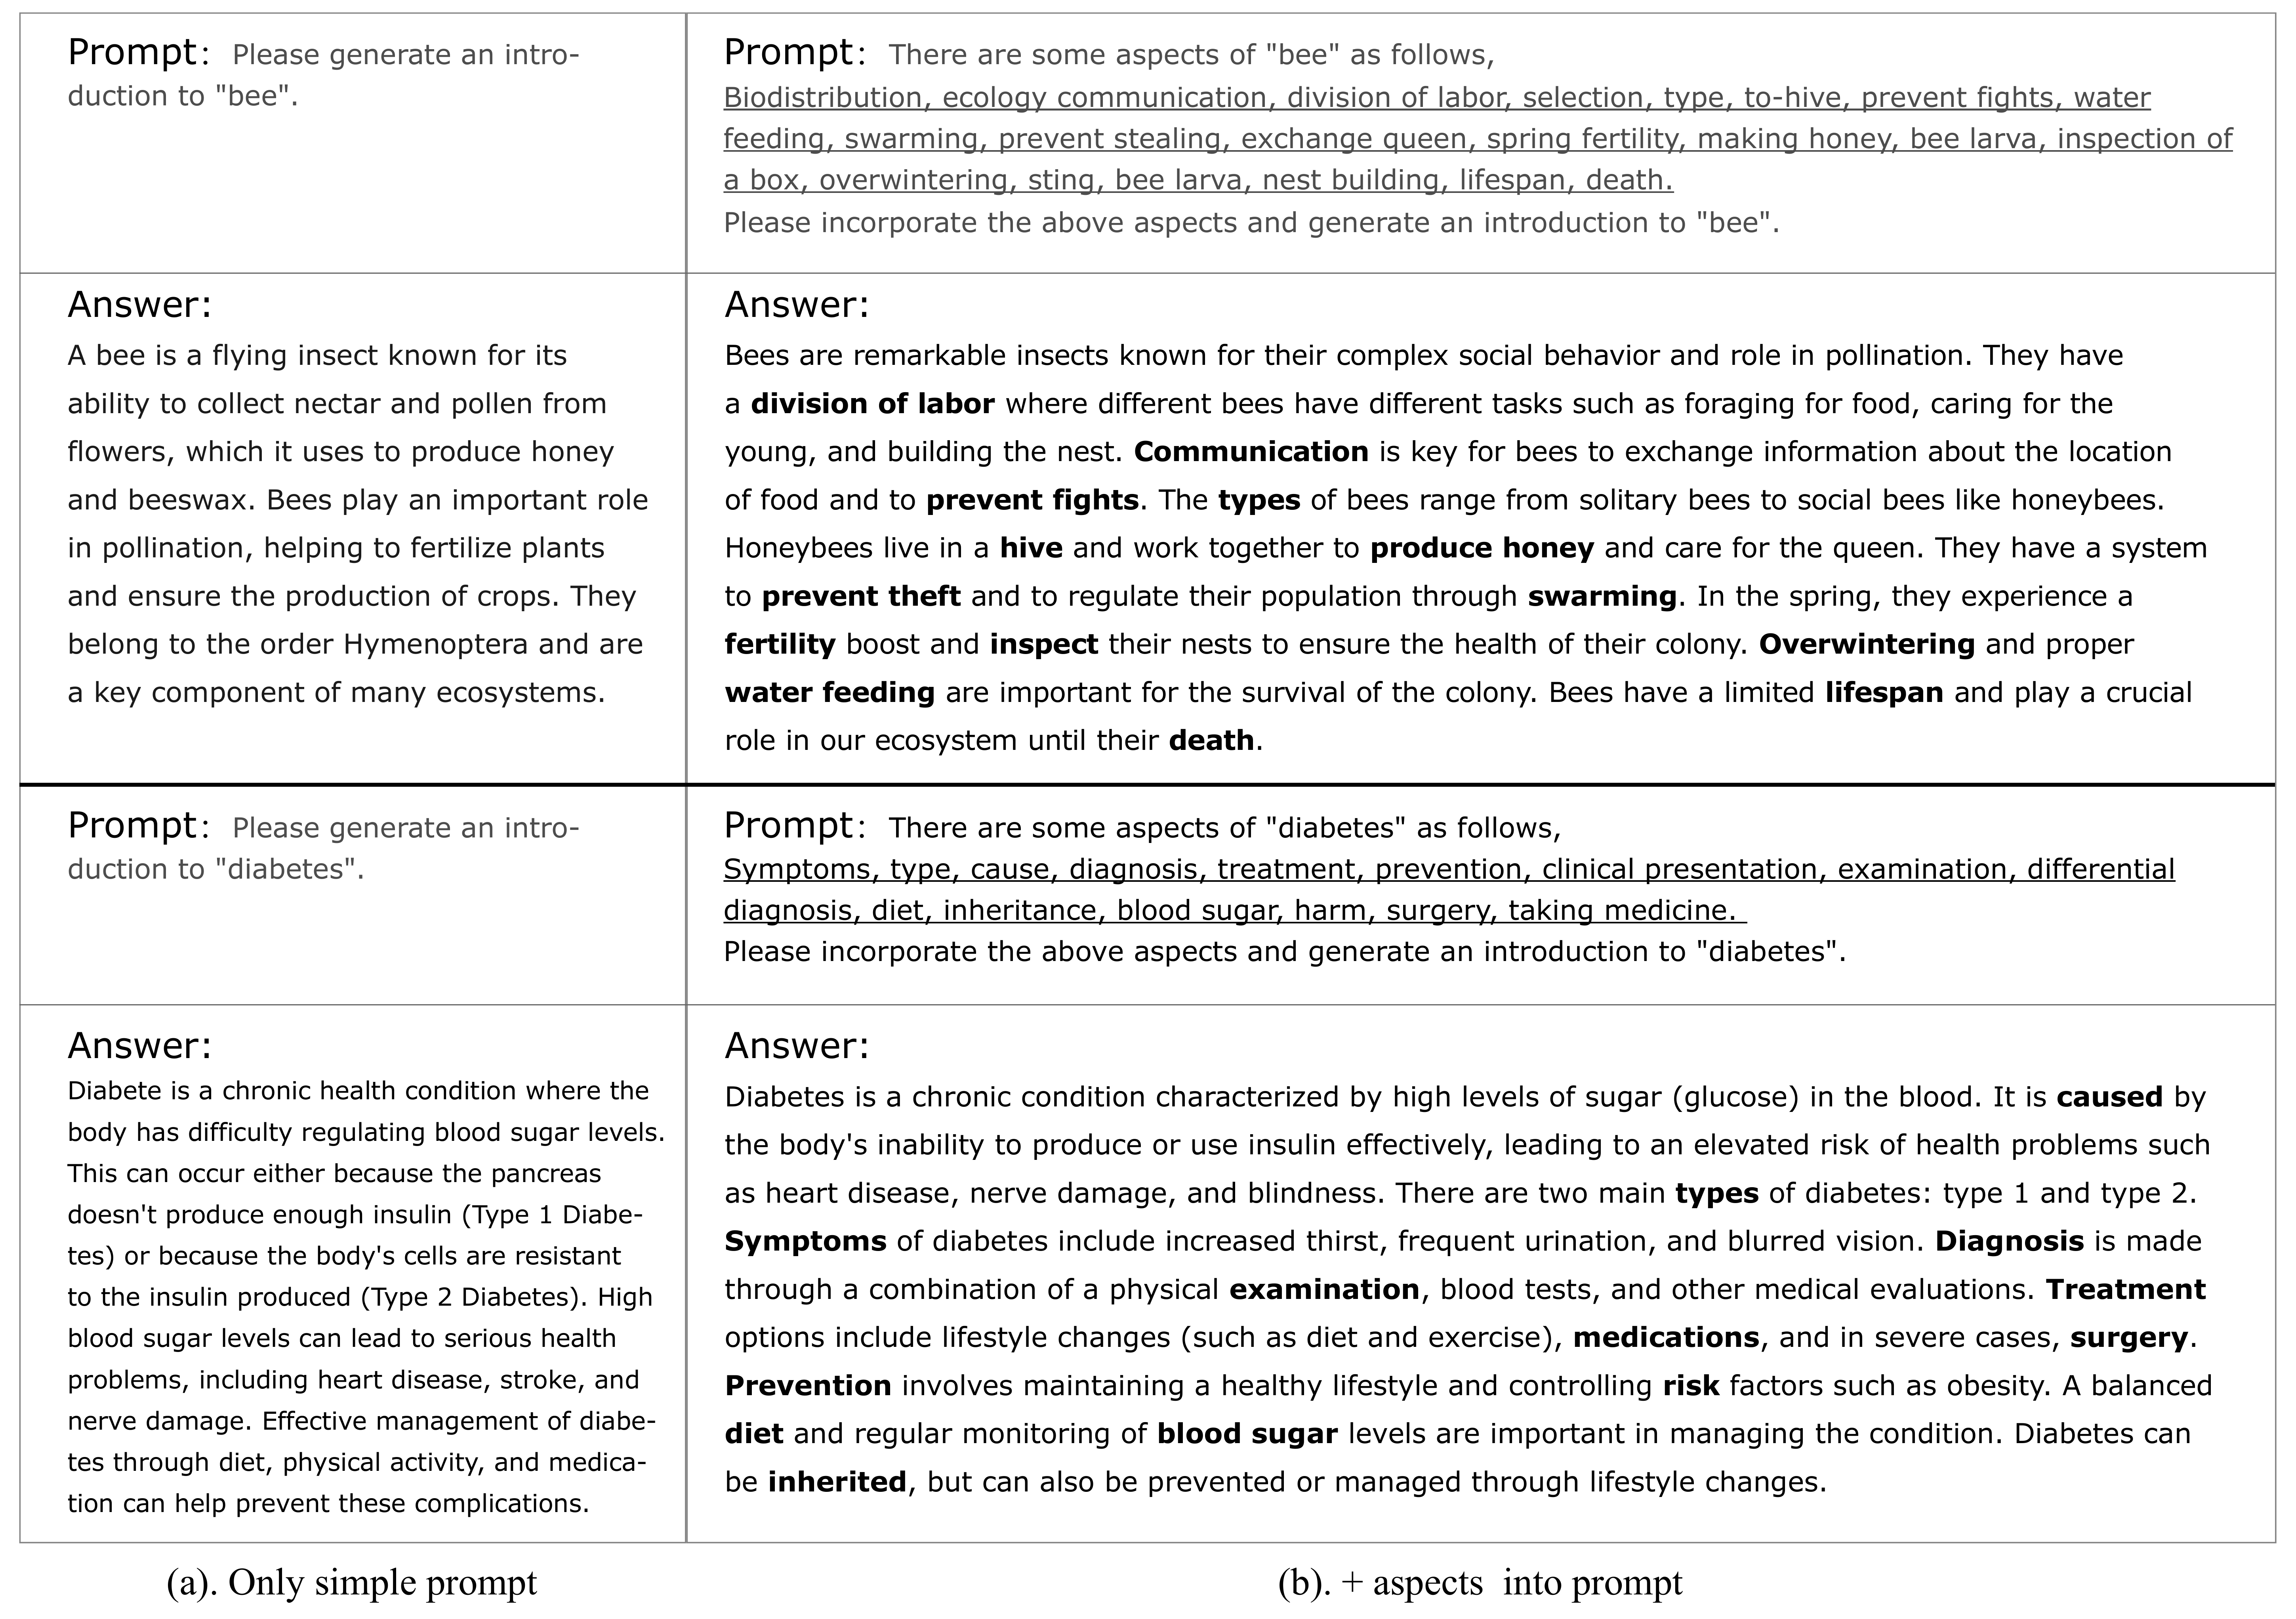}
\caption{Case of how Kuaipedia can help  ChatGPT generate more professional introductions. }\label{fig:chatgpt-case1}
\end{figure*}

\begin{figure*}[h]
\centering
\includegraphics[width=1.0\textwidth]{images/chatgpt-case2-full.pdf}
\caption{Factuality case of how Kuaipedia benefits the generation of ChatGPT. }\label{fig:chatgpt-case2-full}
\end{figure*}

\begin{figure*}[h]
\centering
\includegraphics[height=1.3\textwidth]{}
\caption{More cases of how Kuaipedia help image generation. }
\label{fig:image-gen1}
\end{figure*}

\begin{figure*}[h]
\centering
\includegraphics[height=1.3\textwidth]{}
\caption{More cases of how Kuaipedia help image generation. }
\label{fig:image-gen2}
\end{figure*}

\begin{figure*}[h]
\centering
\includegraphics[height=0.5\textwidth]{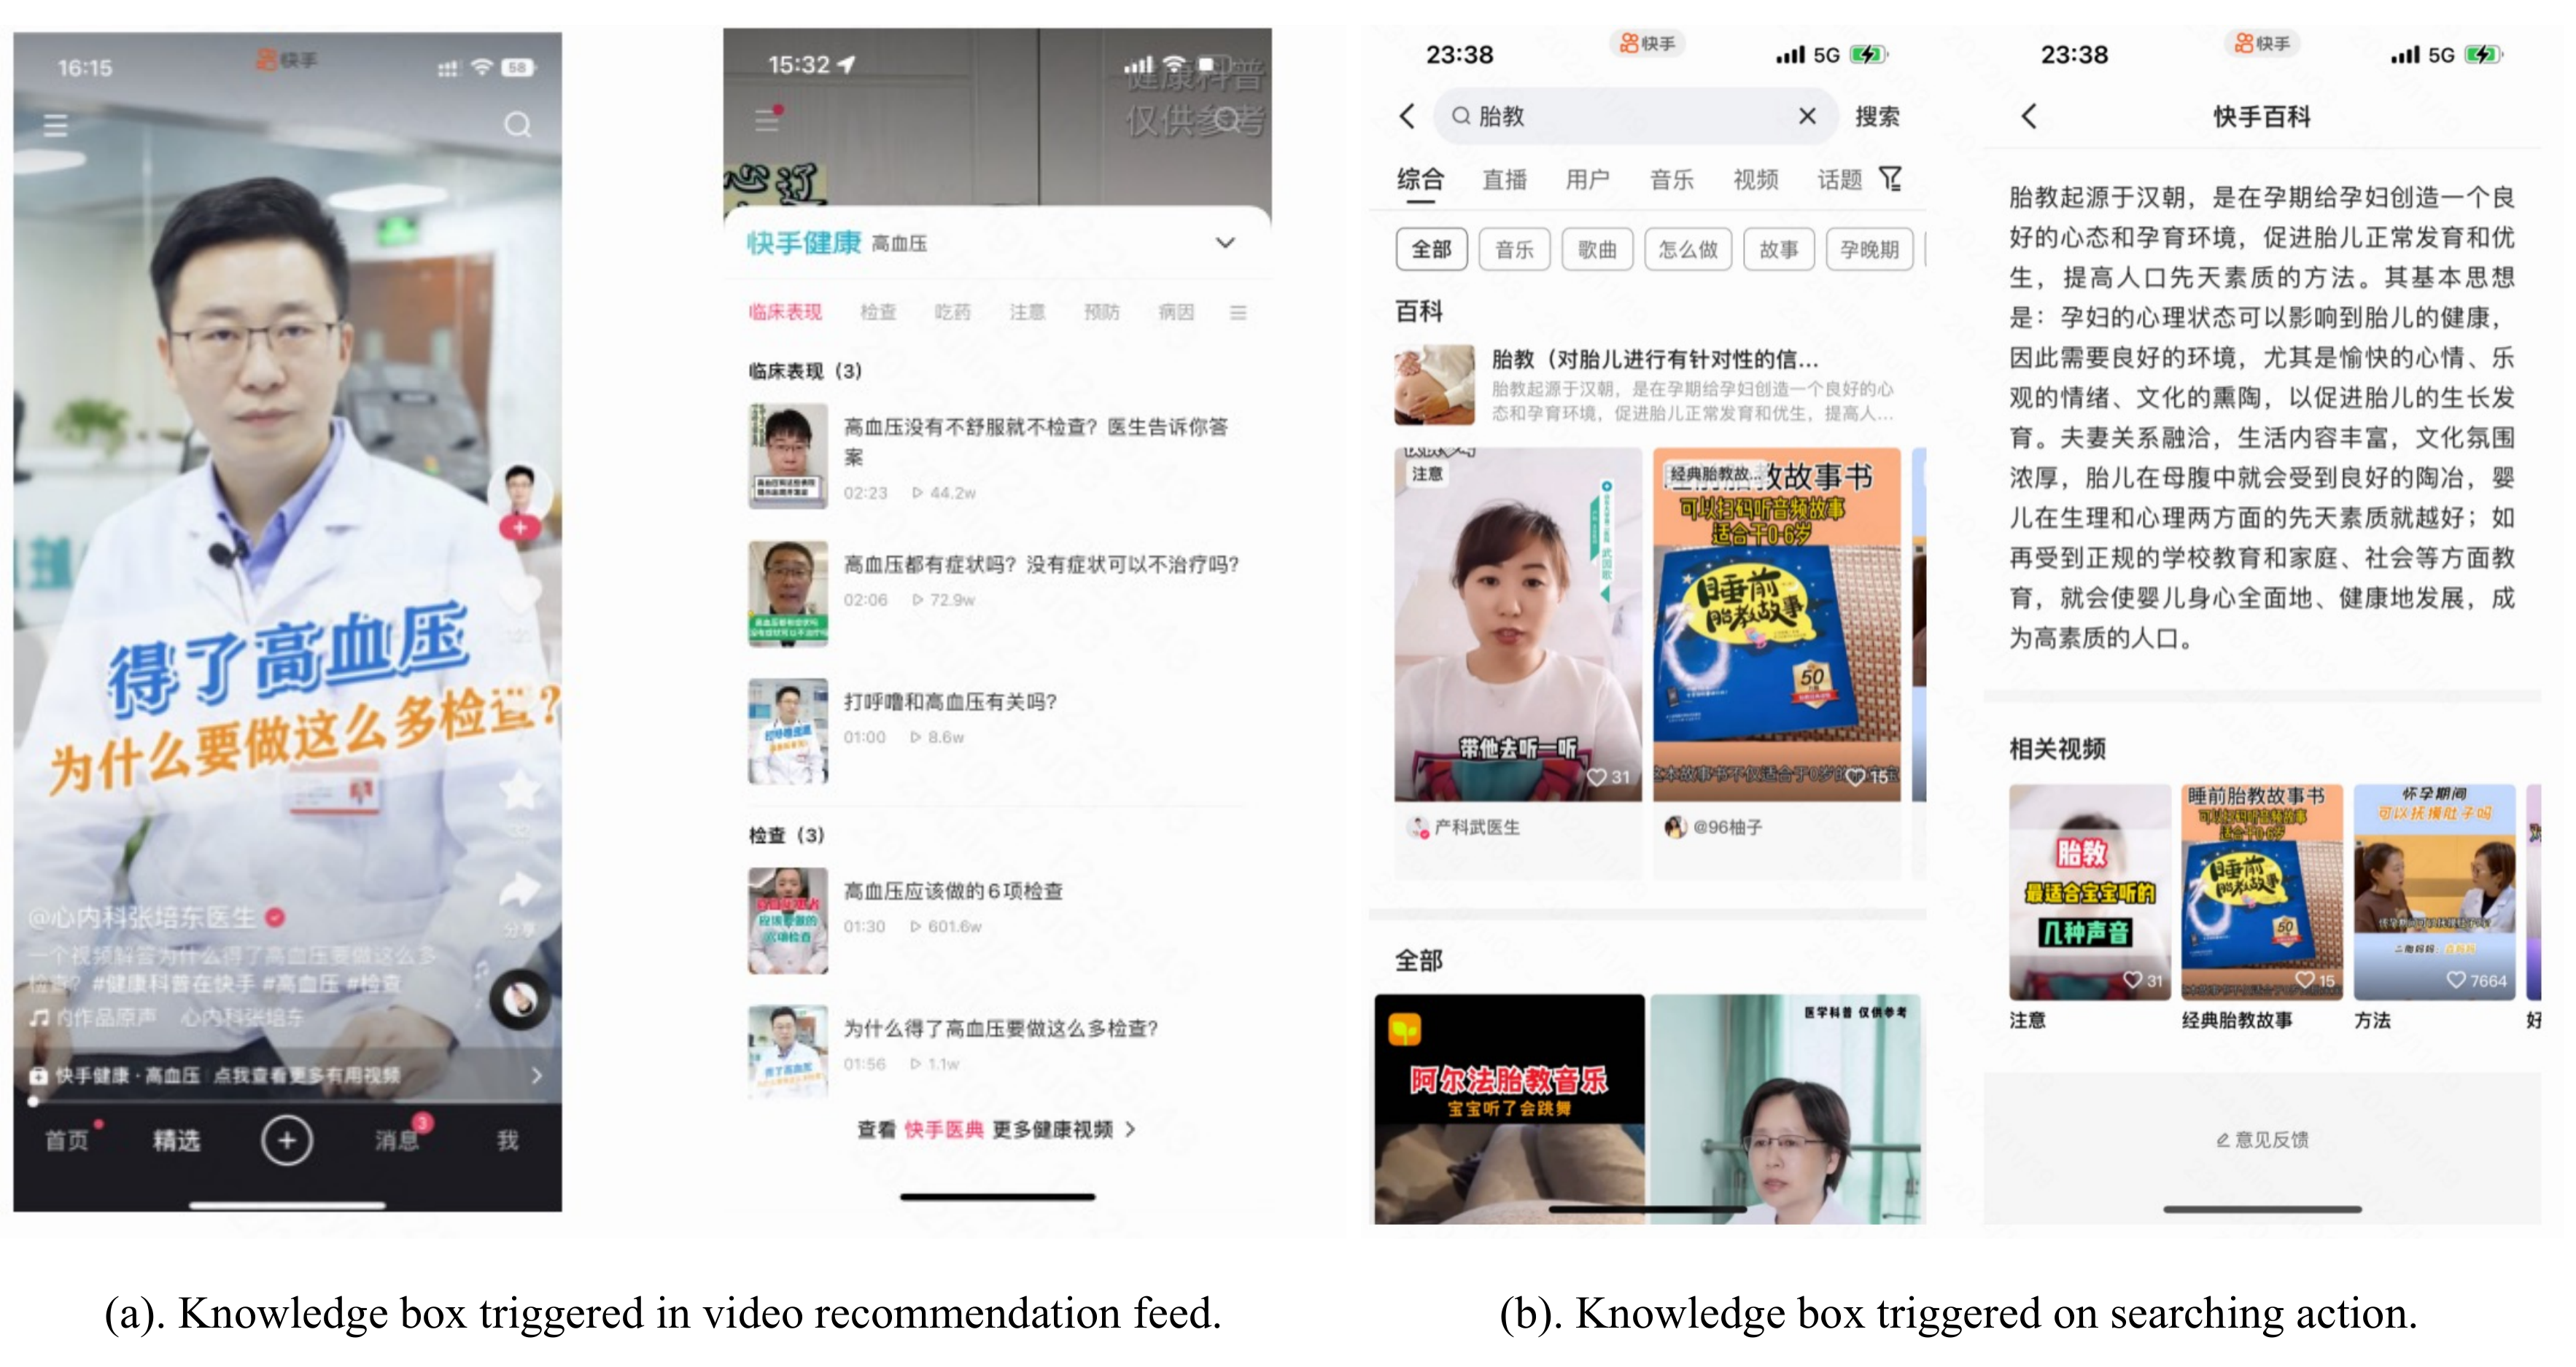}
\caption{Real-time application of Kuaipedia.}
\label{fig:app1}
\end{figure*}

\section{Supplementary Case Study}

\subsection{More cases of Item-aspect pairs in Kuaipedia} \label{more-pairs-case}
In this section, we demonstrate further examples of item-aspect pairs in Kuaipedia, covering a wide range of topics including education, technology, finance, products, sports, and locations. As shown in Figure \ref{fig:aspect-case-appendix} the breadth of these cases serves to highlight the versatility of Kuaipedia in capturing information about diverse subjects. Further examples will be made available when the Kuaipedia public website launches~\footnote{We have uploaded a video clip to show how our Kuaipeida demo works just like wikipedia website}.

\subsection{ChatGPT Factuality Improvement} \label{factuality-case}

In Figure \ref{fig:chatgpt-case2-full}, we showcase the ten responses generated by the ChatGPT model to provide a comprehensive overview of its capabilities and performance. The figure allows us to analyze and evaluate the outputs in greater detail. When posed with the question "Can all bees sting?" ten times, the ChatGPT model consistently replied with "Yes." However, this answer is not entirely accurate as male bees lack stingers and are therefore incapable of stinging. To rectify this issue, the prompt was revised by incorporating descriptive information about the entity in question. The incorporation of additional information related to the item results in a more diverse and potentially accurate set of answers. Our results demonstrate that the highest accuracy was achieved when the top-ranked video about "bees sting" was combined with several OCR frames and added to the input prompt. This result highlights the potential for incorporating multimodal information from Kuaipedia to enhance the accuracy of ChatGPT's responses.

\subsection{ChatGPT Professionaliy Improvement} \label{professionaliy-case}
Kuaipedia can significantly enhance the professionalism of ChatGPT's answers. As an example, we present two cases in Figure \ref{fig:chatgpt-case1} where Kuaipedia proves to be of great help. Firstly, when discussing the topic of bees, ChatGPT typically generates short and succinct descriptions. However, with the incorporation of Kuaipedia's insightful aspects, ChatGPT can produce a more comprehensive scientific article that covers all the relevant topics people may be interested in regarding bees. The same scenario applies in the second case of debates. Despite the occasional mistakes, ChatGPT's answers are more professional, providing a comprehensive and well-structured argument.

\subsection{Image Generation Improvement} \label{img-gen-case}
We present additional cases in Figures \ref{fig:image-gen1} and \ref{fig:image-gen2} to demonstrate the effectiveness of Kuaipedia in improving the performance of image generation models such as Dalle·E and Midjourney. The first column in both figures displays the input of only the item-aspect pair text prompts, the second column adds the ASR text of a corresponding video, and the third column adds the video frames.
Our results show that the image generation models struggled to generate meaningful outputs for most of the "how-to" prompts, and often only generated images of the entity. However, adding the step-by-step ASR text improved the models' ability to generate step-by-step images that explain the "how-to" scenario. The addition of video frames in the prompts also reduced the difficulty of generating images compared to using only item-aspect text.

\section{Real-time application} \label{real-time-app}
We have implemented a real-time functional application on the Kuaishou App. The first application (as shown in Figure \ref{fig:app1}(a)) is integrated into the video recommendation feed, displaying a bottom bar that appears when a video is grounded to Kuaipedia items. By clicking the bottom bar, a ``knowledge box'' is triggered, presenting information about the related items, aspects and associated videos. The second application  (as shown in Figure \ref{fig:app1} (b)) is for searching purposes, where the ``knowledge box'' of Kuaipedia is displayed on the results page of the user's search actions.
